# Supplementary material for: Direct Zernike Coefficient Prediction from Point Spread Functions and Extended Images using Deep Learning
Source: arXiv:2404.15231 source file (2024-04-24)
Supplement: Supplementary file 1 [file supplement.pdf]

# Appendix A

## Subset of results on the simulated PSF dataset

a)

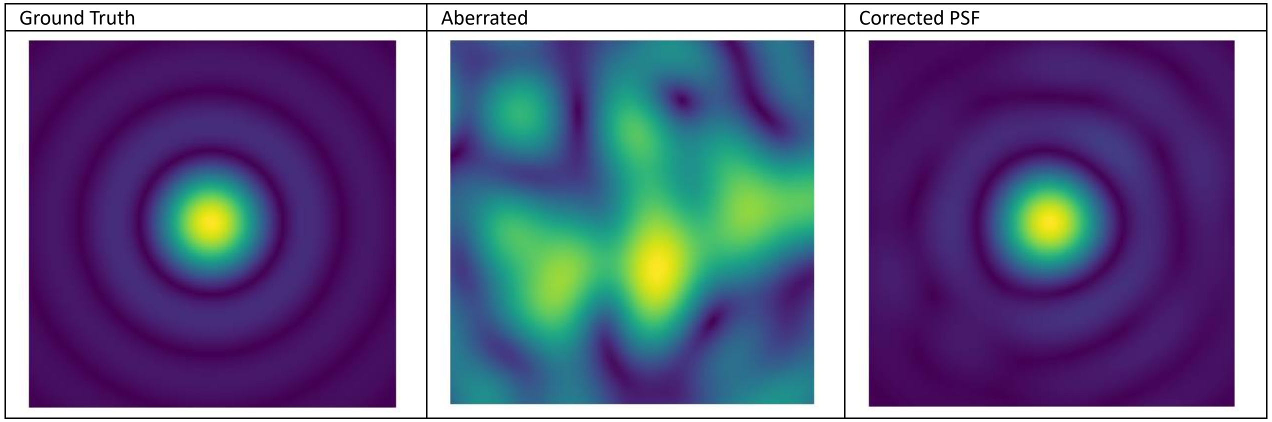


b)

| | |
|---|---|
| **PSNR** | 32.03 |
| **SSIM** | 0.8947 |

c)

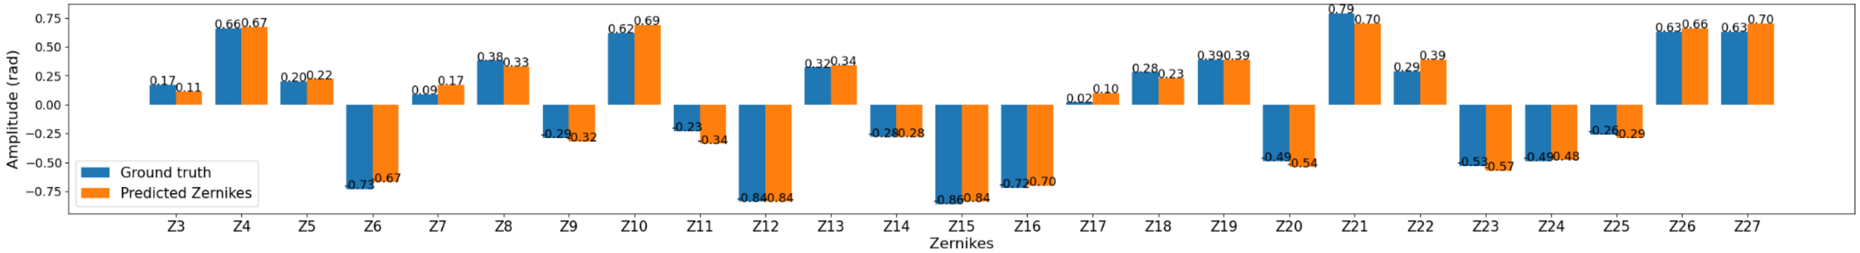


Figure A1: An example of the results on a simulated PSF with aberration. a) shows the ground truth, aberrated PSF image and the corrected image is calculated from the residual aberration (Ground truth Zernike values minus Predicted Zernikes) re-applied to the ground truth image. b) shows the PSNR and SSIM metrics measured between the ground truth and the corrected images. c) shows the ground truth and predicted Zernike coefficients in a bar graph.

a)

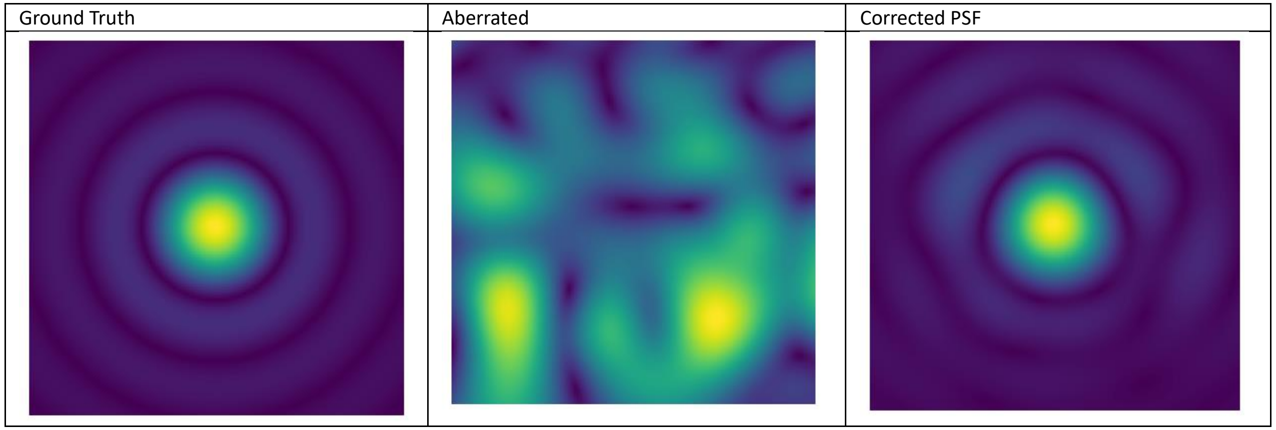


b)

| | |
|---|---|
| **PSNR** | 30.40 |
| **SSIM** | 0.8528 |

c)

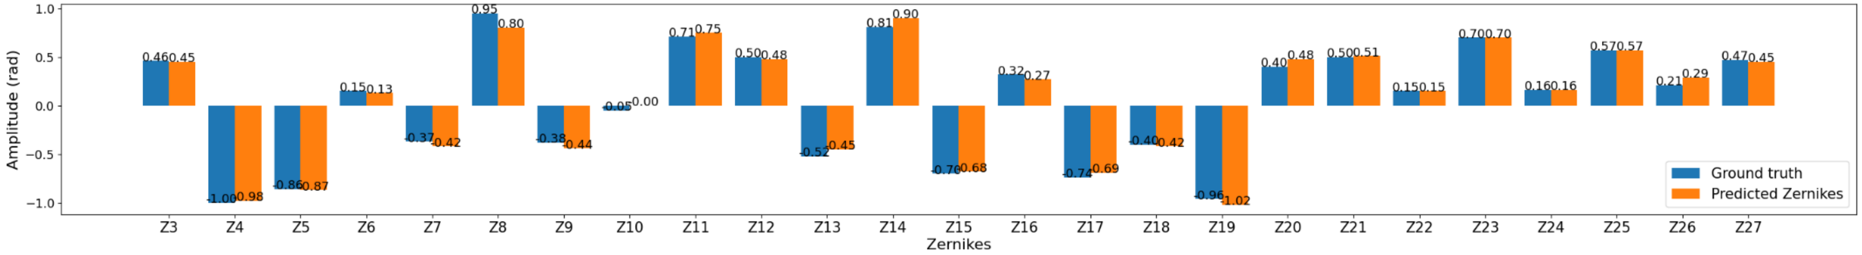


Figure A2: An example of the results on a simulated PSF with aberration. a) shows the ground truth, aberrated PSF image and the corrected image is calculated from the residual aberration (Ground truth Zernike values minus Predicted Zernikes) re-applied to the ground truth image. b) shows the PSNR and SSIM metrics measured between the ground truth and the corrected images. c) shows the ground truth and predicted Zernike coefficients in a bar graph.

a)

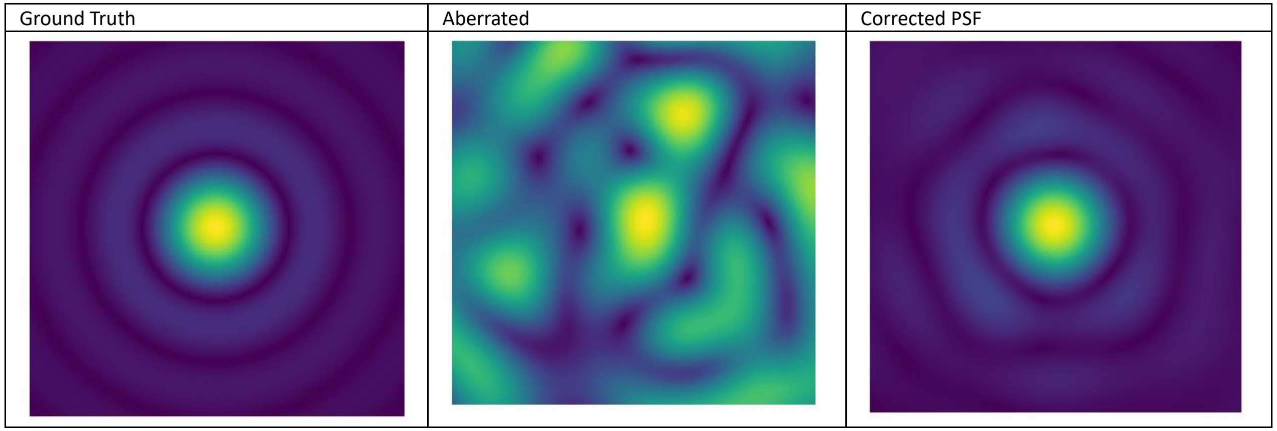


b)

| | |
|---|---|
| **PSNR** | 32.03 |
| **SSIM** | 0.8754 |

c)

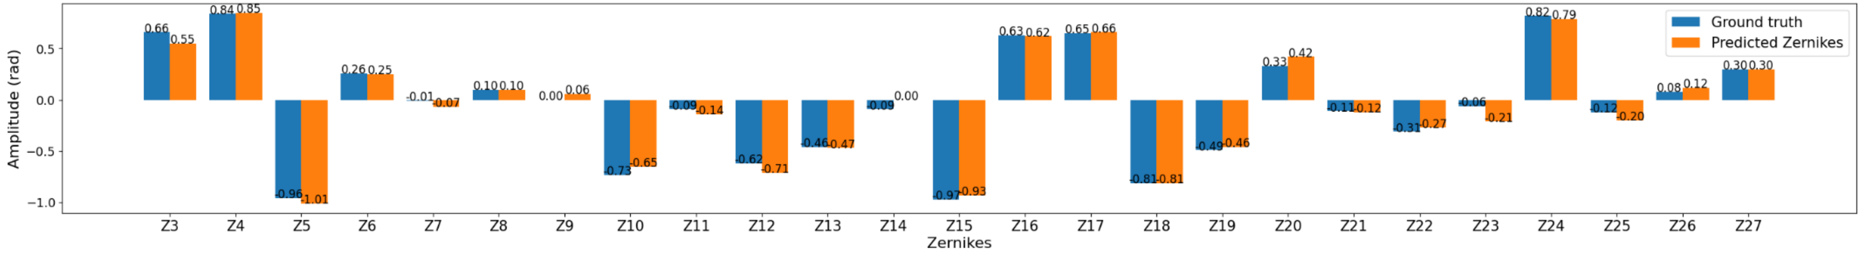


Figure A3: An example of the results on a simulated PSF with aberration. a) shows the ground truth, aberrated PSF image and the corrected image is calculated from the residual aberration (Ground truth Zernike values minus Predicted Zernikes) re-applied to the ground truth image. b) shows the PSNR and SSIM metrics measured between the ground truth and the corrected images. c) shows the ground truth and predicted Zernike coefficients in a bar graph.

a)

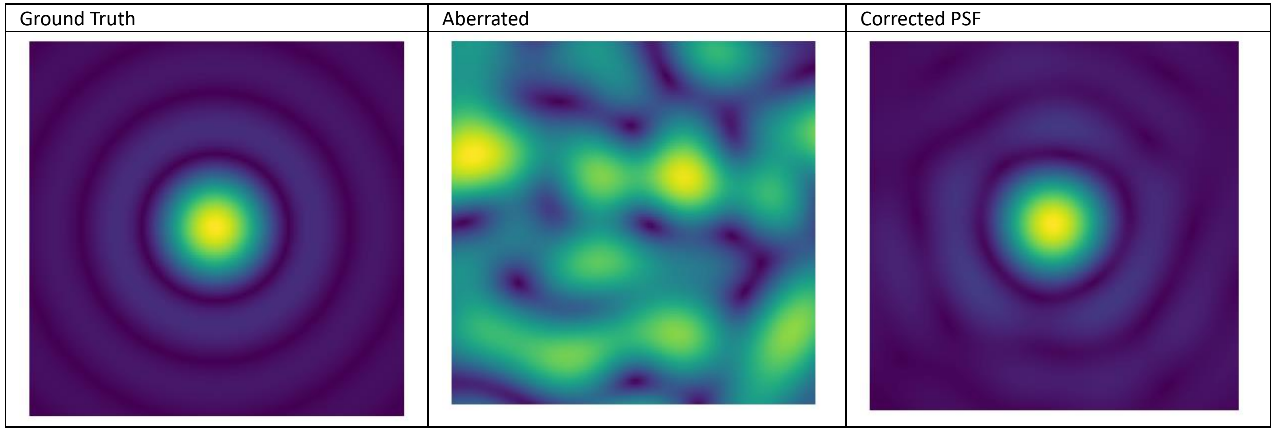


b)

| | |
|---|---|
| **PSNR** | 32.54 |
| **SSIM** | 0.8805 |

c)

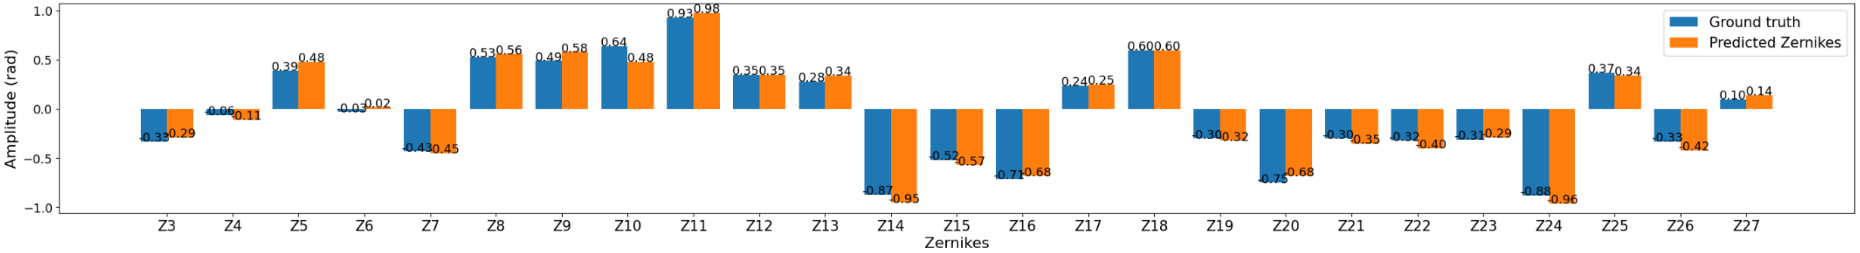


Figure A4: An example of the results on a simulated PSF with aberration. a) shows the ground truth, aberrated PSF image and the corrected image is calculated from the residual aberration (Ground truth Zernike values minus Predicted Zernikes) re-applied to the ground truth image. b) shows the PSNR and SSIM metrics measured between the ground truth and the corrected images. c) shows the ground truth and predicted Zernike coefficients in a bar graph.

## Appendix B

### Subset of results on the simulated extended 2D sample dataset

a)

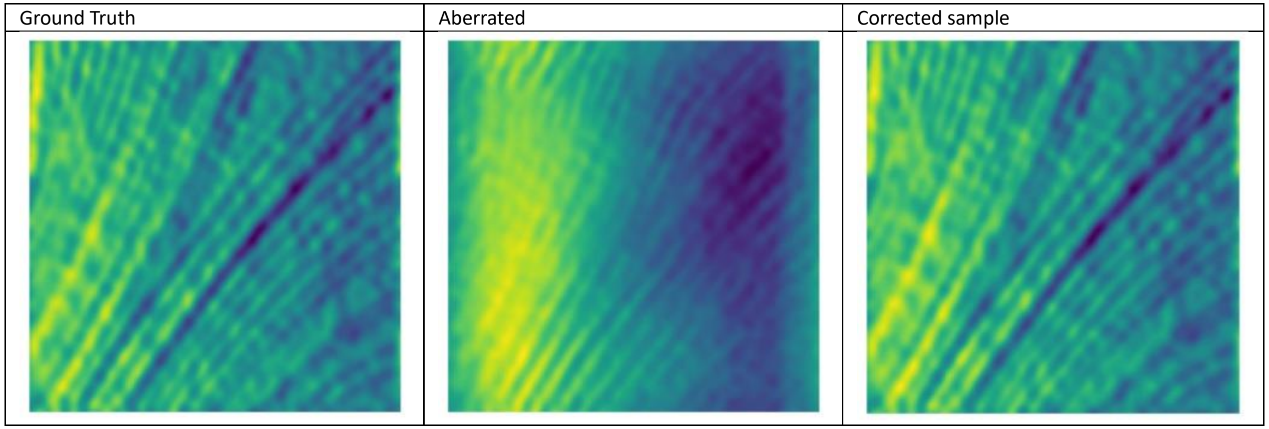


b)

| | |
|---|---|
| **PSNR** | 50.03 |
| **SSIM** | 0.9956 |

c)

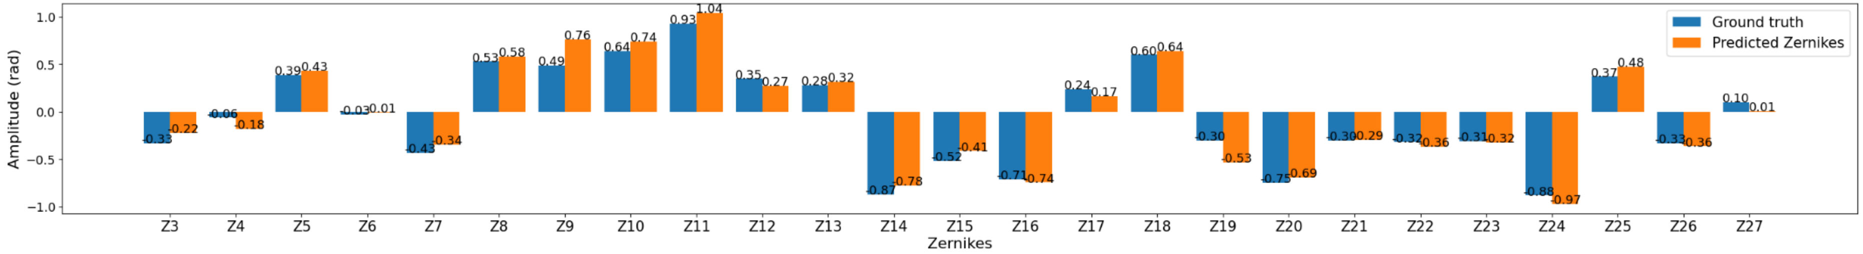


Figure B1: An example of the results on an extended 2D sample with aberration. a) shows the ground truth, aberrated image and the the corrected image is calculated from the residual aberration (Ground truth Zernike values minus Predicted Zernikes) re-applied to the ground truth image. b) shows the PSNR and SSIM metrics measured between the ground truth and the corrected images. c) shows the ground truth and predicted Zernike coefficients in a bar graph.

a)

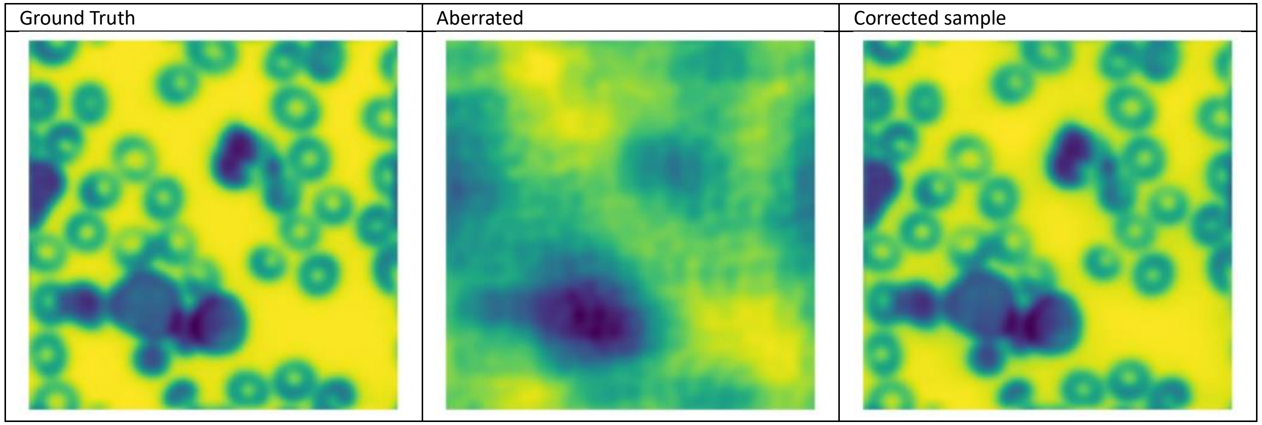


b)

| | |
|---|---|
| **PSNR** | 43.44 |
| **SSIM** | 0.9944 |

c)

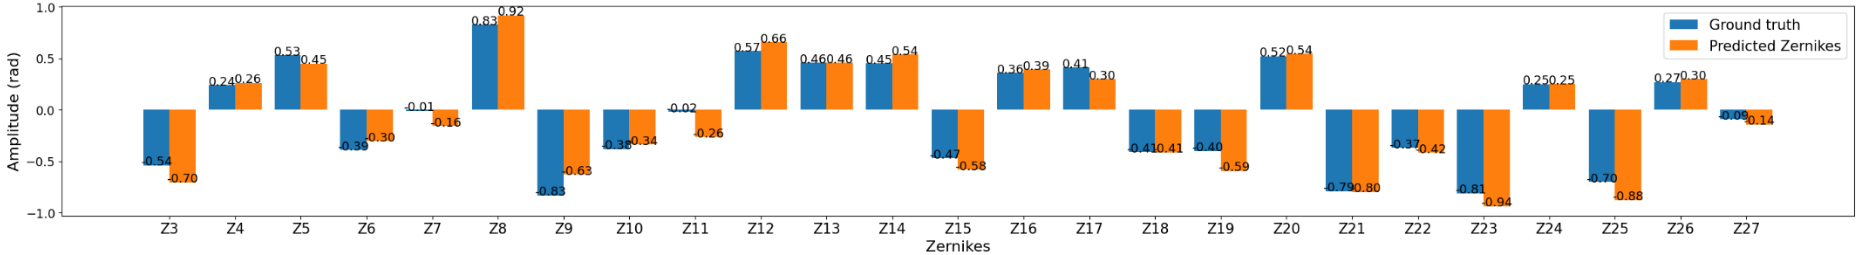


Figure B2: An example of the results on an extended 2D sample with aberration. a) shows the ground truth, aberrated image and the corrected image is calculated from the residual aberration (Ground truth Zernike values minus Predicted Zernikes) re-applied to the ground truth image. b) shows the PSNR and SSIM metrics measured between the ground truth and the corrected images. c) shows the ground truth and predicted Zernike coefficients in a bar graph.

a)

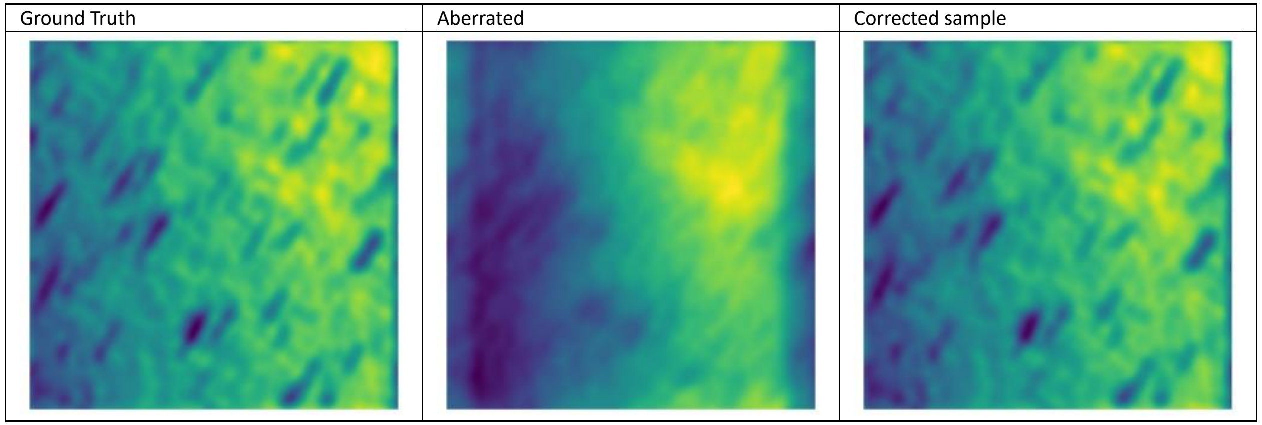


b)

| | |
|---|---|
| **PSNR** | 46.01 |
| **SSIM** | 0.9936 |

c)

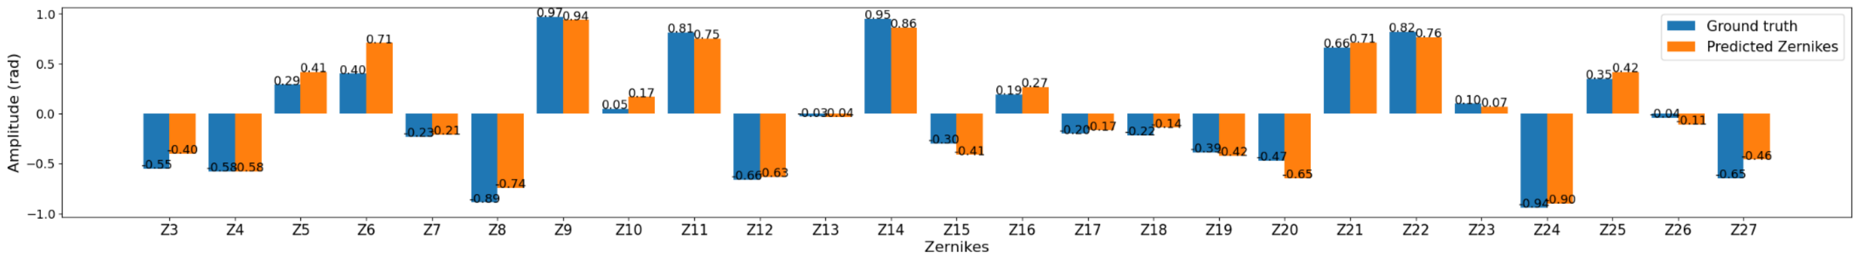


Figure B3: An example of the results on an extended 2D sample with aberration. a) shows the ground truth, aberrated image and the the corrected image is calculated from the residual aberration (Ground truth Zernike values minus Predicted Zernikes) re-applied to the ground truth image. b) shows the PSNR and SSIM metrics measured between the ground truth and the corrected images. c) shows the ground truth and predicted Zernike coefficients in a bar graph.

a)

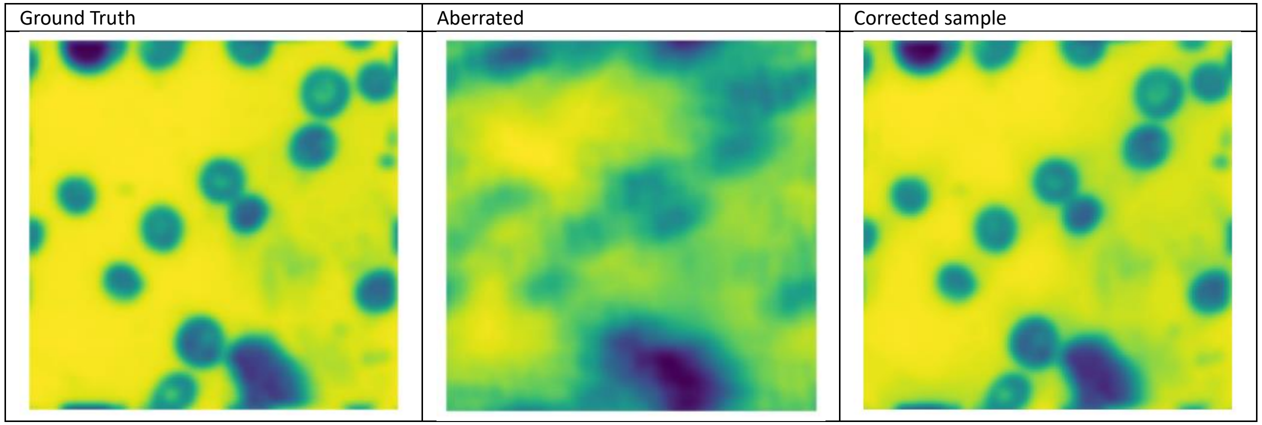


b)

| | |
|---|---|
| **PSNR** | 32.42 |
| **SSIM** | 0.9845 |

c)

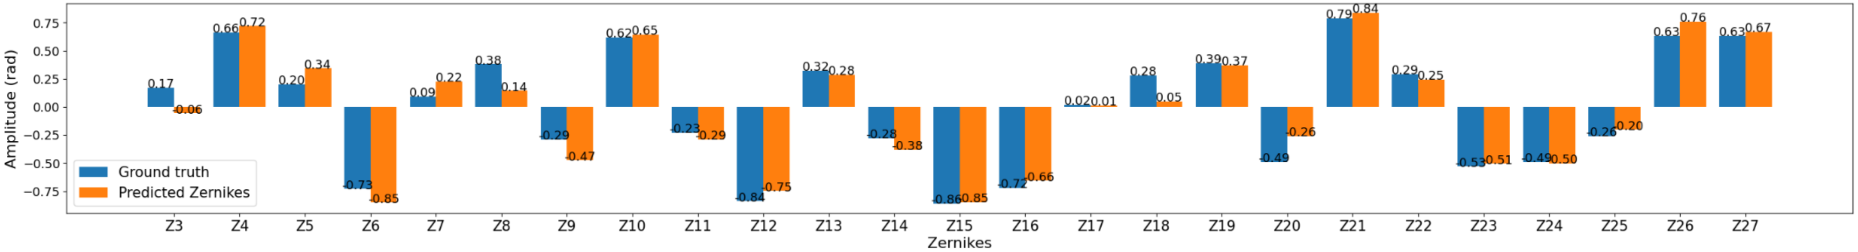


Figure B4: An example of the results on an extended 2D sample with aberration. a) shows the ground truth, aberrated image and the the corrected image is calculated from the residual aberration (Ground truth Zernike values minus Predicted Zernikes) re-applied to the ground truth image. b) shows the PSNR and SSIM metrics measured between the ground truth and the corrected images. c) shows the ground truth and predicted Zernike coefficients in a bar graph.
