# Supplementary material for: Direct Zernike Coefficient Prediction from Point Spread Functions and Extended Images using Deep Learning
Source: arXiv:2404.15231 source file (2024-04-24)
Supplement: Supplementary file 2 [file supplementary.tex]

\documentclass[fleqn,10pt]{wlscirep}
\usepackage{pdfpages}
\begin{document}
\includepdf[pages=-,pagecommand={},landscape=true]{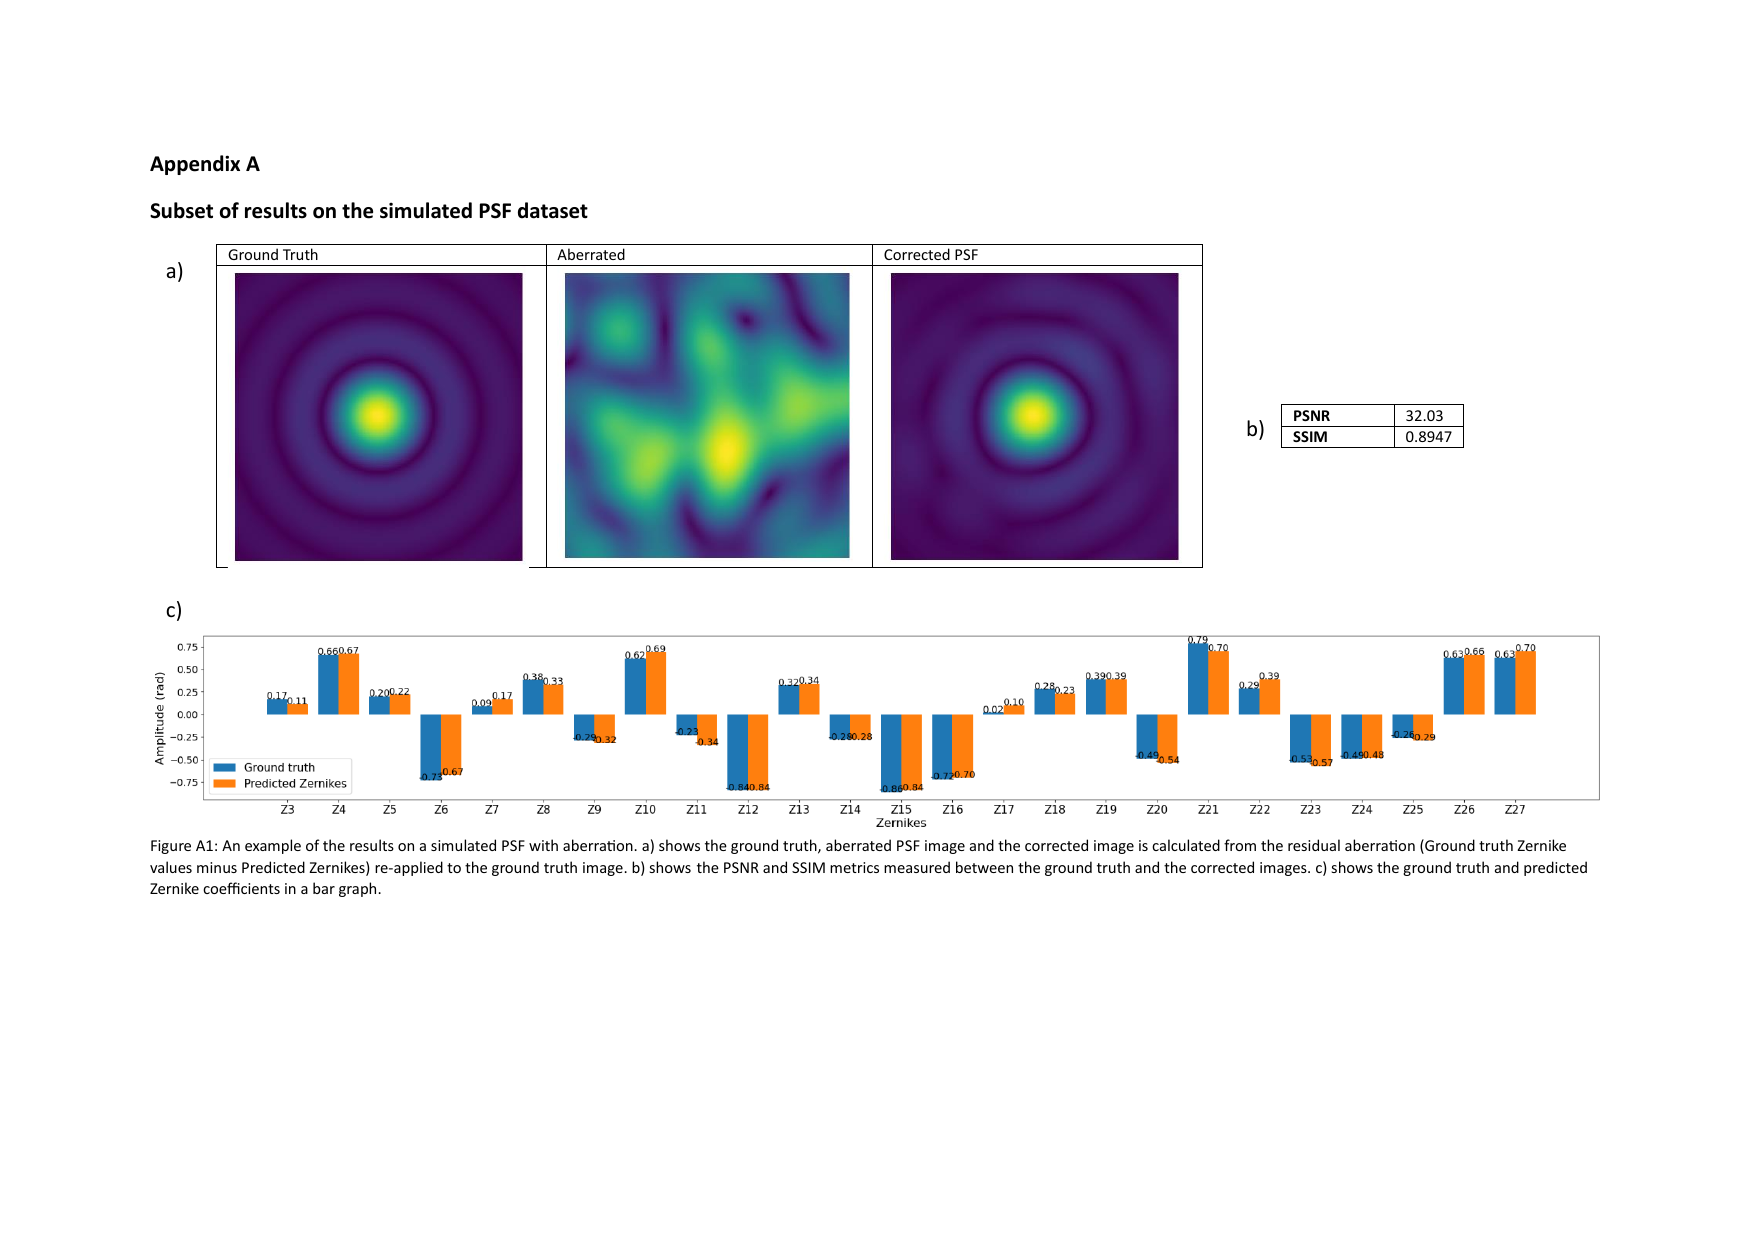}
\end{document}
